# Supplementary material for: A Model for Attribute Based Role-Role Assignment (ARRA)
Source: arXiv:1706.10274 source file (2018-12-24)
Supplement: Supplementary file 1 [file appendix.tex]

\begin{figure}[t]
 \centering
 \includegraphics[scale=0.25]{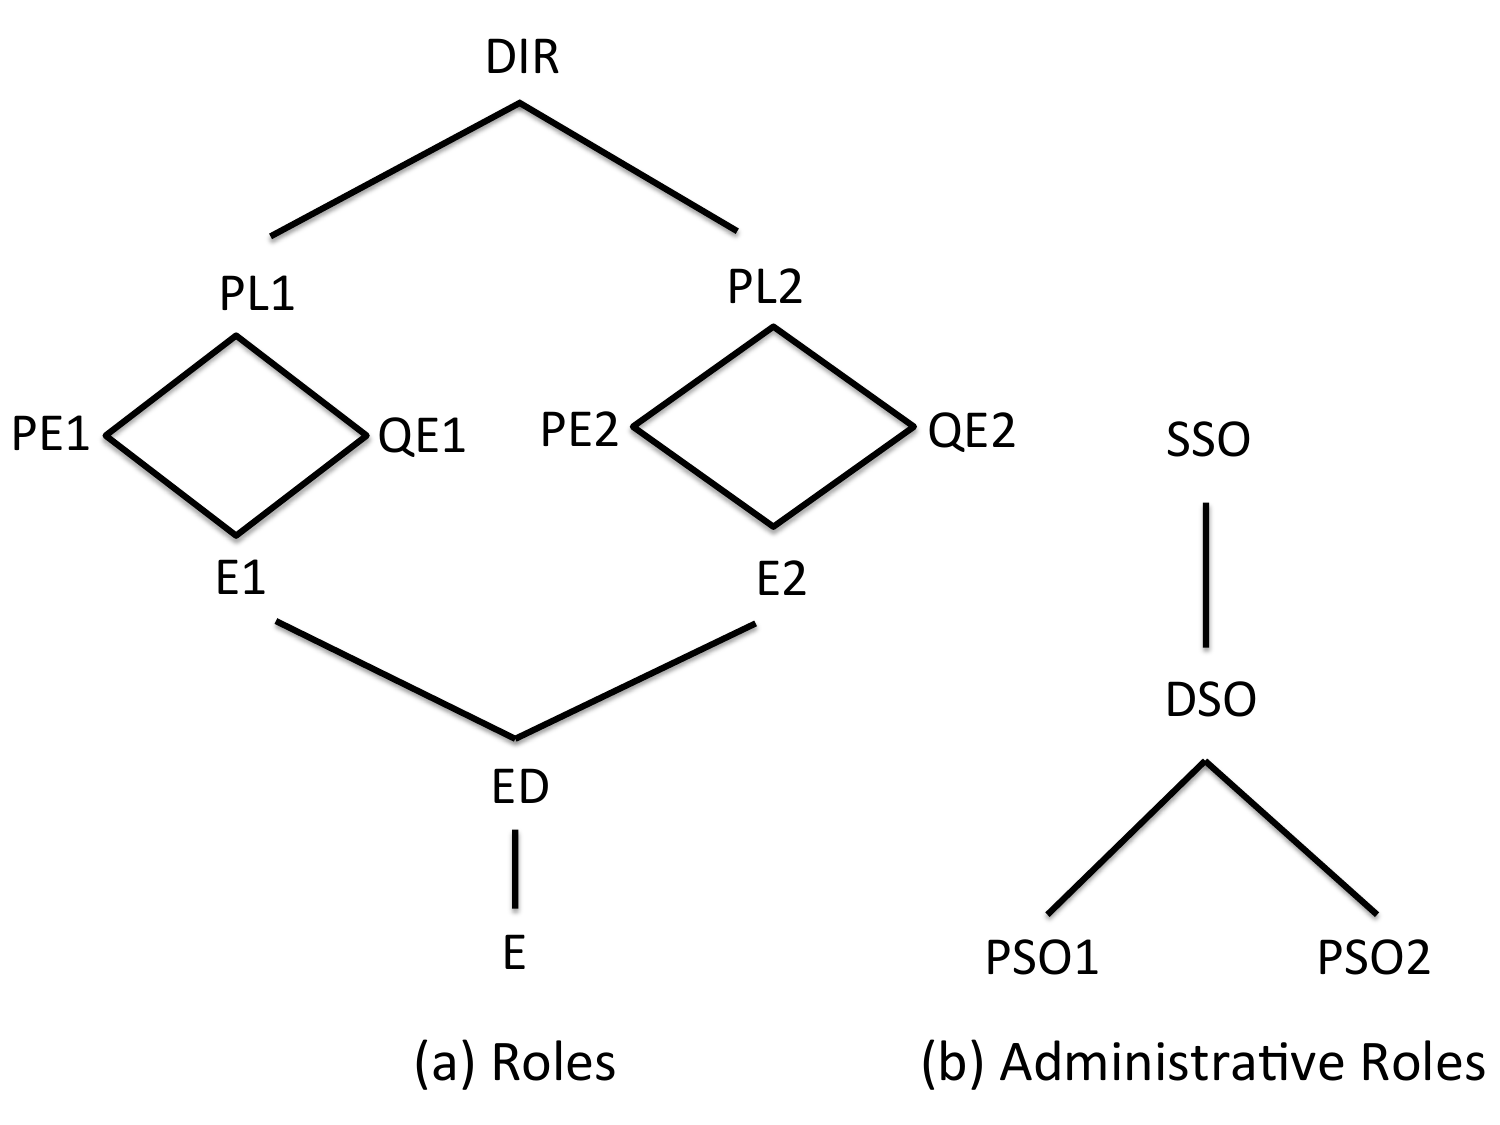}
 \caption{Role and Administrative Role Hierarchies in RRA97}
 \label{fig:roleh}
\end{figure}

\appendices
\label{appendix}
\section{Mapping an Example RRA97 Instance in ARRA}
\label{urra97-appendix}

\noindent

\section{Mapping an Example Instance of \\
UARBAC's RRA in ARRA}\label{rrau-appendix}

\noindent
\textbf{An Example UARBAC's RRA Instance:}\\
\underline{RBAC schema}
\begin{itemize}
\item \it{C} = \{\textsf{role}\}
\item \it{OBJS}(\textsf{user}) = \textbf{USERS}, \it{OBJS}(\textsf{role}) = \textbf{ROLES}
% \item \it{AM}(\textsf{user}) = \{\textsf{empower, admin}\},
\item \it{AM}(\textsf{role}) = \{\textsf{grant, empower, admin}\}
\end{itemize}
\underline{RBAC state}
\begin{itemize}
\item \it{\U} = \it{OBJ}(\textsf{user}) = \{\textbf{u\textsubscript1, u\textsubscript2, u\textsubscript3, u\textsubscript4}\} 
\item \it{\R} = \it{OBJ}(\textsf{role})= \{\textbf{r\textsubscript{1}, r\textsubscript{2}, r\textsubscript3}\} % $\cup$ \textbf{sso}, where \textbf{sso} is a reserved role called Senior Security Officer.
\item \it{P} = [\textsf{role}, \textbf{r\textsubscript1}, \textsf{grant}], [\textsf{role}, \textbf{r\textsubscript1}, \textsf{empower}], [\textsf{role}, \textbf{r\textsubscript1}, \textsf{admin}], [\textsf{role}, \textbf{r\textsubscript2}, \textsf{grant}], [\textsf{role}, \textbf{r\textsubscript2}, \textsf{empower}], [\textsf{role}, \textbf{r\textsubscript2}, \textsf{admin}], [\textsf{role}, \textbf{r\textsubscript3}, \textsf{grant}], [\textsf{role}, \textbf{r\textsubscript3}, \textsf{empower}], [\textsf{role}, \textbf{r\textsubscript3}, \textsf{admin}], {[\textsf{role}, \textsf{grant}], [\textsf{role, empower}], [\textsf{role, admin}]\}}
%\item \it{\UA} = \{(\textbf{u\textsubscript1, r\textsubscript1}), (\textbf{u\textsubscript2, r\textsubscript1}), (\textbf{u\textsubscript2, r\textsubscript2}), (\textbf{u\textsubscript2, r\textsubscript3}), (\textbf{u\textsubscript3, r\textsubscript3}), (\textbf{u\textsubscript4, r\textsubscript2})\}
\item \it{\RH} = \{<\textbf{r\textsubscript2, r\textsubscript3}>\}
\end{itemize}
\noindent
\underline{Administrative permissions of UARBAC's RRA}\\
Following is the list of administrative permissions each user has for role-role assignment:
\begin{itemize}
\item authorized\_perms[\textbf{u\textsubscript1}]  = \{{[\textsf{role}, \textbf{r\textsubscript1}, \textsf{grant}],
\item[] \stab {[\textsf{role}, \textbf{r\textsubscript2}, \textsf{admin}]}, [\textsf{role}, \textbf{r\textsubscript2}, \textsf{empower}]}, 
\item[] \stab {[\textsf{role}, \textbf{r\textsubscript3}, \textsf{admin}]}\}

\item authorized\_perms[\textbf{u\textsubscript2}]  = \{[\textsf{role}, \textbf{r\textsubscript1}, \textsf{admin}],
\item[] \stab {[\textsf{role}, \textbf{r\textsubscript1}, \textsf{empower}]}, [\textsf{role}, \textbf{r\textsubscript2}, \textsf{empower}], 
\item[] \stab {[\textsf{role}, \textbf{r\textsubscript3}, \textsf{grant}]}\}
\item authorized\_perms[\textbf{u\textsubscript3}] = \{[\textsf{role, admin}]\}
\item authorized\_perms[\textbf{u\textsubscript4}] = \{[\textsf{role, grant}], \item[] \stab {[\textsf{role, empower}]}, {[\textsf{role, admin}]}\}
\end{itemize}
\underline{Role-role assignment condition}\\
One can perform following operation to assign a role \textbf{r\textsubscript1} to another role \textbf{r\textsubscript2}.
\begin{itemize}
\item grantRoleToRole(\textbf{r\textsubscript{1}, r\textsubscript{2}}) 
\end{itemize}
To perform this operation one needs one of the following two permissions:
\begin{itemize}
\item {[\textsf{role}, \textbf{r\textsubscript1}, \textsf{grant}]} and {[\textsf{role}, \textbf{r\textsubscript2}, \textsf{empower}]} or,
\item {[\textsf{role}, \textsf{grant}]} and {[\textsf{role}, \textbf{r\textsubscript2}, \textsf{empower}]} or,
\item {[\textsf{role}, \textbf{r\textsubscript1}, \textsf{grant}]} and {[\textsf{role}, \textsf{empower}]} or,
\item {[\textsf{role}, \textsf{grant}]} and {[\textsf{role}, \textsf{empower}]}
\end{itemize}
\underline{Condition for revoking a role from another role}\\
To revoke a role \textbf{r\textsubscript2} from a role \textbf{r\textsubscript3}, admin user performs following operation.
\begin{itemize}
\item revokeRoleFromUser(\textbf{r\textsubscript{2}, r\textsubscript{3}}) 
\end{itemize}
To conduct this operation one needs one of the following options:
\begin{itemize}
\item {[\textsf{role}, \textbf{r\textsubscript2}, \textsf{grant}] and [\textsf{role}, \textbf{r\textsubscript3}, \textsf{empower}]}
\item {[\textsf{role}, \textbf{r\textsubscript2}, \textsf{admin}]} 
\item {[\textsf{role}, \textbf{r\textsubscript3}, \textsf{admin}]}
\item {[\textsf{role}, \textsf{admin}]}
\end{itemize}

\vspace{0.19cm}
\noindent
%
%%%%%%%%%%%%%%%%%%%%%%%%%%%%%%%%%%%%%%%%%%%%%%%%%%%%%%%%%%%%%%%%%%%%%      URA-UARBAC      %%%%%%%%%%%%%%%%%%%%%%%%%%%%%%%%%%%%%%%%%%%%%%%%%%%%%%%%%%%%%%%%%%%%%%%%%%%%%%%%%%%%%%%%%%%%%%%%%%%%%%%%%%%%%%%%%%%%%%%%%%%%%%%%%%%%%%%
\subsubsection{Equivalent ARRA instance UARBAC's RRA}
\begin{itemize}
%\item \U\ = \{\textbf{u\textsubscript{1}, u\textsubscript{2}, u\textsubscript{3}, u\textsubscript4}\}
\item \AU\ = \{\textbf{u\textsubscript{1}, u\textsubscript{2}, u\textsubscript{3}, u\textsubscript4}\}, \OP\ = \{\textbf{assign, revoke}\}
\item \R\ = \{\textbf{r\textsubscript{1}, r\textsubscript{2}, r\textsubscript3}\}, \AUA\ = \{\}
\item \RH\ = \{<\textbf{r\textsubscript2, r\textsubscript3}>\}
\item \AATT\ = \{\textit{grantAuth, empowerAuth, adminAuth, roleClassAuth}\}, \ARATT\ = \{\}, \RATT\ = \{\}
%\item[] \tab class\_grantAuth, class\_empowerAuth,
%\item[] \tab class\_adminAuth}\}
\item \scope(\textit{grantAuth}) = \{\textbf{r\textsubscript{1}, r\textsubscript{2}, r\textsubscript3}\}
\item[] attType(\it{grantAuth}) = set, 
\item[] \isord(\it{grantAuth}) = \R\textsuperscript{{A}}, H\textsubscript{\it{grantAuth}} = \RH\textsuperscript{{A}}

\item \it{grantAuth}(\textbf{u\textsubscript{1}}) = \{\textbf{r\textsubscript1}\}, \it{grantAuth}(\textbf{u\textsubscript{2}}) = \{\textbf{r\textsubscript3}\},
\item[] \it{grantAuth}(\textbf{u\textsubscript{3}}) = \{\}, \it{grantAuth}(\textbf{u\textsubscript{4}}) = \{\}

\item \scope(\textit{empowerAuth}) = \{\textbf{r\textsubscript{1}, r\textsubscript{2}, r\textsubscript3}\}
\item[] attType(\it{empowerAuth}) = set, 
\item[] \isord(\it{empowerAuth}) = \R\textsuperscript{{A}}
\item[] H\textsubscript{\it{empowerAuth}} = \RH\textsuperscript{{A}}

\item \it{empowerAuth}(\textbf{u\textsubscript{1}}) = \{\textbf{r\textsubscript2}\}, 
\item[]\it{empowerAuth}(\textbf{u\textsubscript{2}}) = \{\textbf{r\textsubscript1, r\textsubscript2}\},
\item[] \it{empowerAuth}(\textbf{u\textsubscript{3}}) = \{\}, \it{empowerAuth}(\textbf{u\textsubscript{4}}) = \{\}

\item \scope(\textit{adminAuth}) = \{\textbf{r\textsubscript{1}, r\textsubscript{2}, r\textsubscript3}\}
\item[] attType(\it{adminAuth}) = set, 
\item[] \isord(\it{adminAuth}) = \R\textsuperscript{{A}},
\item[] H\textsubscript{\it{adminAuth}} = \RH\textsuperscript{{A}}

\item \it{adminAuth}(\textbf{u\textsubscript{1}}) = \{\textbf{r\textsubscript2, r\textsubscript3}\}, 
\item[]\it{adminAuth}(\textbf{u\textsubscript{2}}) = \{\textbf{r\textsubscript1}\},
\item[] \it{adminAuth}(\textbf{u\textsubscript{3}}) = \{\}, \it{adminAuth}(\textbf{u\textsubscript{4}}) = \{\}
%%---------------------------------------------- class level perms
\item \scope(\textit{roleClassAuth}) = \it{AM}(\textsf{role})
\item[] attType(\it{roleClassAuth}) = set, 
\item[] \isord(\it{roleClassAuth}) = False, 
\item[] H\textsubscript{\it{roleClassAuth}} = $\phi$

\item \it{roleClassAuth}(\textbf{u\textsubscript{1}}) = \{\}, \it{roleClassAuth}(\textbf{u\textsubscript{2}}) = \{\textbf{}\},
\item[] \it{roleClassAuth}(\textbf{u\textsubscript{3}}) = \{\textsf{admin}\},
\item[] \it{roleClassAuth}(\textbf{u\textsubscript{4}}) = \{\textsf{grant, empower, admin}\}

%\item \scope(\textit{class\_grantAuth}) = \{\textsf{role}\}
%\item[] attType(\it{class\_grantAuth}) = set, 
%\item[] \isord(\it{class\_grantAuth}) = False, 
%\item[] H\textsubscript{\it{class\_grantAuth}} = $\phi$
%
%\item \it{class\_grantAuth}(\textbf{u\textsubscript{1}}) = \{\}, 
%\item[] \it{class\_grantAuth}(\textbf{u\textsubscript{2}}) = \{\textbf{}\},
%\item[] \it{class\_grantAuth}(\textbf{u\textsubscript{3}}) = \{\},
%\item[] \it{class\_grantAuth}(\textbf{u\textsubscript{4}}) = \{\textsf{role}\}
%
%\item \scope(\textit{class\_empowerAuth}) = \{\textsf{role}\}
%\item[] attType(\it{class\_empowerAuth}) = set, 
%\item[] \isord(\it{class\_empowerAuth}) = False,
%\item[] H\textsubscript{\it{class\_empowerAuth}} = $\phi$
%
%\item \it{class\_empowerAuth}(\textbf{u\textsubscript{1}}) = \{\}, 
%\item[]\it{class\_empowerAuth}(\textbf{u\textsubscript{2}}) = \{\textbf{}\},
%\item[] \it{class\_empowerAuth}(\textbf{u\textsubscript{3}}) = \{\}, 
%\item[] \it{class\_empowerAuth}(\textbf{u\textsubscript{4}}) = \{\textsf{role}\}
%
%\item \scope(\textit{class\_adminAuth}) = \{\textsf{role}\}
%\item[] attType(\it{class\_adminAuth}) = set, 
%\item[] \isord(\it{class\_adminAuth}) = False,
%\item[] H\textsubscript{\it{class\_adminAuth}} = $\phi$
%
%\item \it{class\_adminAuth}(\textbf{u\textsubscript{1}}) = \{\textbf{}\}, 
%\item[]\it{class\_adminAuth}(\textbf{u\textsubscript{2}}) = \{\textbf{}\},
%\item[] \it{class\_adminAuth}(\textbf{u\textsubscript{3}}) = \{\}, 
%\item[] \it{class\_grantAuth}(\textbf{u\textsubscript{4}}) = \{\textsf{role}\}

\end{itemize}
For each \it{op} in \OP, authorization rule to assign/revoke role-role can be expressed as follows:\\
To assign any regular role \it{r\textsubscript1} $\in$ \R\ to regular role \it{r\textsubscript2} $\in$ \R,\\
-- {\isauth}U\textsubscript{\textbf{assign}}(\it{au\textsubscript{}} : \AU, \it{r\textsubscript1} : \R, \\
\hspace*{0.3cm}\it{r\textsubscript2} : \R) $\equiv$ \\
\hspace*{0.3cm}(\it{r\textsubscript{1}} $\in$ \it{grantAuth}(\it{au\textsubscript{}}) $\wedge$ \it{r\textsubscript2} $\in$ \it{empowerAuth}(\it{au\textsubscript{}})) $\vee$\\
\hspace*{0.3cm}(\it{r\textsubscript{1}} $\in$ \it{grantAuth}(\it{au\textsubscript{}}) $\wedge$ \textsf{empower} \\
\hspace*{0.3cm}$\in$ \it{roleClassAuth}(\it{au\textsubscript{}})) $\vee$ 
(\textsf{grant} $\in$ \it{roleClassAuth}(\it{au\textsubscript{}}) $\wedge$ \\
\hspace*{0.3cm}\it{r\textsubscript2} $\in$ \it{empowerAuth}(\it{au\textsubscript{}})) $\vee$ (\textsf{grant} $\in$ \it{roleClassAuth}(\it{au\textsubscript{}}) \\
\hspace*{0.3cm}$\wedge$ \textsf{empower} $\in$ \it{roleClassAuth}(\it{au\textsubscript{}}))
 
 \vspace{0.17cm}
 \noindent
 To revoke any regular role \it{r\textsubscript1} $\in$ \R\ from another regular role \it{r\textsubscript2} $\in$ \R,\\
-- {\isauth}U\textsubscript{\textbf{revoke}}(\it{au\textsubscript1} : \AU, \it{r\textsubscript1} : \R,\\
\hspace*{0.3cm}\it{r\textsubscript2} : \R) $\equiv$ \\
\hspace*{0.3cm}(\it{r\textsubscript{1}} $\in$ \it{grantAuth}(\it{au\textsubscript{}}) $\wedge$ \it{r\textsubscript2} $\in$ \it{empowerAuth}(\it{au\textsubscript{}})) $\vee$\\
\hspace*{0.3cm}\it{r\textsubscript{1}} $\in$ \it{adminAuth}(\it{au\textsubscript{}}) $\vee$ \it{r\textsubscript{2}} $\in$ \it{adminAuth}(\it{au\textsubscript{}}) $\vee$\\
\hspace*{0.3cm}\textsf{admin} $\in$ \it{roleClassAuth}(\it{au})
